# Supplementary material for: Semi-Parametric Retrieval via Binary Bag-of-Tokens Index
Source: arXiv:2405.01924 source file (2025-03-06)
Supplement: Supplementary file 1 [file 2-ablation.tex]

\section{Details of Ablation Study}
\label{sec:appendix-ablation}
In this section, we detail the methodology behind our ablation study.
First, we assess the impact of removing specific components we proposed on overall performance.
Initially, we explore the effects of excluding the in-training negative retrieval, opting instead to use the standard BM25 negatives for the entirety of the training process. 
This configuration is referred to as ``w/o retrieved neg''.
We further investigate the influence of omitting additional negatives. To maintain the same number of passages in each mini-batch despite this removal, we double the batch size. While this approach still allows for in-batch negatives to be used for contrastive learning, it essentially equates to employing random negative samples for each query. We term this setting as ``w/o neg''.
While exclude the semi-parameter objective, the $\beta$ search become non-functional, we reference the performance of the $\rm{VDR}$  as an indicator, and term this setting as ``w/o SP objective''.
 
We also assess the effect of the configuration during in-training retrieval.
We investigate the impact of negative sample hardness on model performance. To this end, we manipulate the value of $m$, referred to as ``w/ retrieved neg (m)''. 
Our negative samples are randomly selected from the top-$m$ passages identified by \oursb, with the value of $m$ indirectly determining the difficulty of these negatives. A smaller $m$ indicates a higher difficulty of the negative samples retrieved by \oursb. We conduct evaluations at $m=1$ and $m=100$ to assess how varying the difficulty of negative samples influences retrieval performance.
Moreover, we explore the influence of the source of retrieved negatives by switching the retrieval corpus from Wikipedia to MS MARCO, denoted as ``w/ retrieved neg (MARCO)''. We also conduct an ablation study where the size of the Wikipedia corpus is reduced to 8.8 million passages, matching the size of MS MARCO, to isolate the effects of corpus size on retrieval performance. This setting is referred to as ``w/ retrieved neg (WIKI 8m)''.
