# Supplementary material for: Semi-Parametric Retrieval via Binary Bag-of-Tokens Index
Source: arXiv:2405.01924 source file (2025-03-06)
Supplement: Supplementary file 2 [file 0-limitation.tex]

\section{Limitations}
\label{sec:appendix-limit}
\paragraph{Multi-modality.} 
While $\rm{VDR}$~\cite{zhou2024retrievalbased} has proven effective in both text-to-text and cross-modal retrieval settings, our work builds upon it with a focus on semi-parametric objectives. However, this design limitation prevents our framework from extending to cross-modal scenarios. This limitation arises from our reliance on binary token representation for both query and passage side, which is inherent to textual data only.

\paragraph{Vocabulary.} 
Our lexical retrieval harnesses the effectiveness of masked language model (MLMs), with the vocabulary predefined by the tokenizer and the MLM itself. While our work utilizes a BERT-based model as the encoder, which typically has a relatively smaller vocabulary size of 30k, multilingual encoders often have a larger vocabulary. This can increase latency due to the computational overhead of projection to the vocabulary space, as observed in the latency gap between our approach and $\rm{DPR}$.
