# Supplementary material for: Semi-Parametric Retrieval via Binary Bag-of-Tokens Index
Source: arXiv:2405.01924 source file (2025-03-06)
Supplement: Supplementary file 3 [file 6-sparsity.tex]

\section{Amounts of Activation}
\label{sec:appendix-sparsity}

\begin{table*}[ht]
\centering
\scalebox{0.7}{
\begin{tabular}{|l|ccccc|l|}
\hline
\multirow{2}{*}{Model} & \multicolumn{5}{c|}{Activation of Query} & \multirow{2}{*}{Best} \\ \cline{2-6}
 & 32 & 64 & 128 & 256 & 768 &  \\ \hline
MS MARCO & 34.2 & 34.2 & 34.2 & 34.2 & {\ul \textbf{34.2}} & 34.2 \\ \hline
ArguAna & 53.0 & 53.0 & 53.0 & \textbf{53.0} & 52.0 & 53.0 \\
Climate-FEVER & 17.8 & \textbf{17.9} & 17.6 & 17.1 & 16.6 & 17.9 \\
DBPedia & 38.8 & 39.0 & 39.1 & 39.1 & \textbf{39.3} & 39.3 \\
FEVER & 71.5 & \textbf{71.5} & 71.4 & 71.0 & 70.8 & 71.5 \\
FiQA & 29.6 & 29.7 & \textbf{29.8} & 29.5 & 29.7 & 29.8 \\
HotpotQA & 65.1 & 65.3 & 65.4 & 65.4 & \textbf{65.4} & 65.4 \\
NFCorpus & 33.0 & 33.0 & 33.0 & 33.0 & \textbf{33.0} & 33.0 \\
NQ & 47.7 & 47.7 & 47.7 & 47.7 & \textbf{47.7} & 47.7 \\
SCIDOCS & 15.0 & 15.1 & 15.1 & 15.1 & \textbf{15.1} & 15.1 \\
SciFact & 66.2 & \textbf{66.2} & 65.7 & 65.7 & 65.9 & 66.2 \\
TREC-COVID & 68.0 & 68.0 & 68.0 & 68.0 & \textbf{68.0} & 68.0 \\
Touché-2020 & 29.4 & \textbf{29.7} & 29.3 & 29.1 & 28.6 & 29.7 \\ \hline
Average & 44.6 & 44.7 & 44.6 & 44.5 & 44.3 & 44.7 \\ \hline
\end{tabular}}
\caption{Effectiveness of \oursf~with varying activation amounts. \textbf{Bold} denotes the best query activation amount.}
\label{tab:sparsity}
\end{table*}

We present the effectiveness of \oursf with different amounts of activation $k$ in Table~\ref{tab:sparsity}. Following prior work~\citep{zhou2024retrievalbased}, we report results using the best query activation amount.
