# Supplementary material for: Semi-Parametric Retrieval via Binary Bag-of-Tokens Index
Source: arXiv:2405.01924 source file (2025-03-06)
Supplement: Supplementary file 4 [file cost-effect.tex]

\color{red} 

\section{Cost-Effectiveness Analysis}
\label{sec:cost-effect}

% Table generated by Excel2LaTeX from sheet 'Sheet6'
\begin{table}[htbp]
  \centering
  \caption{Add caption}
  \scalebox{0.7}{
    \begin{tabular}{lcccc}
    \toprule
       & \multicolumn{3}{c}{Cost} & \multirow{2}[4]{*}{effectiveness} \\
\cmidrule{2-4}       & query & passage & total &  \\
\cmidrule{2-5}    \multicolumn{5}{l}{\textit{\textbf{Non-parametric}}} \\
    \quad BM25 & 0  & 0  & 0  &  \\
    \midrule
    \multicolumn{4}{l}{\textit{\textbf{Semi-parametric beta search}}} &  \\
    \quad $\text{SiDR}_{\beta}$ & 3.6k & 0  & 3.6k &  \\
    \midrule
    \multicolumn{5}{l}{\textit{\textbf{Late-parametric}}} \\
    \quad  $\text{SiDR}_{\beta}(m=5)$ & 3.6k & 18k & 18k &  \\
    \quad  $\text{SiDR}_{\beta}(m=20)$ & 3.6k & 72k & 76k &  \\
    \quad  $\text{SiDR}_{\beta}(m=100)$ & 3.6k & 361k & 365k &  \\
    \midrule
    \multicolumn{5}{l}{\textit{\textbf{Full parametric}}} \\
    \quad $\text{SiDR}_{\text{full}}$ & 3.6k & 21m & 21m &  \\
    \bottomrule
    \end{tabular}%
    }
  \label{tab:addlabel}%
\end{table}%
